# Supplementary material for: Disorder effects in correlated topological insulators
Source: arXiv:1608.06634 source file (2016-08-23)
Supplement: Supplementary file 1 [file Supplemental-8-22-16.pdf]

# Supplemental: Disorder effects in correlated topological insulators

Hsiang-Hsuan Hung,[1] Aaron Barr,[1] Emil Prodan,[2] and Gregory A. Fiete[1]

[1] *Department of Physics, The University of Texas at Austin, Austin, TX, 78712, USA*

[2] *Department of Physics, Yeshiva University, New York, NY 10016, USA*

(Dated: August 22, 2016)

## NUMERICAL EVALUATION OF THE CHERN NUMBERS FOR FINITE LATTICES WITH DISORDER

Here we describe how to compute the Chern number of a generic projector $P$ defined on the Hilbert space of a lattice Hamiltonian. We recall that the defining characteristics of a projection are $P^2 = P$ and $P^\dagger = P$. If the projector commutes with the translations, $[T_a, P] = 0$, then it accepts a Bloch-Floquet decomposition:

$$\langle \boldsymbol{x}|P|\boldsymbol{y}\rangle = \int_{\mathbb{T}^2} \frac{\mathrm{d}k}{(2\pi)^2}\, e^{i\boldsymbol{k}\cdot(\boldsymbol{x}-\boldsymbol{y})}\, P_{\boldsymbol{k}} \quad \Leftrightarrow \quad P = \sum_{\boldsymbol{x},\boldsymbol{y}} \int_{\mathbb{T}^2} \frac{\mathrm{d}k}{(2\pi)^2}\, e^{i\boldsymbol{k}\cdot(\boldsymbol{x}-\boldsymbol{y})}\, P_{\boldsymbol{k}} |\boldsymbol{x}\rangle\langle \boldsymbol{y}|, \tag{1}$$

where each of the $P_{\boldsymbol{k}}$ is a finite dimensional projector of dimension equal to the number of orbitals per unit cell. Furthermore, if the matrix elements $\langle \boldsymbol{x}|P|\boldsymbol{y}\rangle$ decay fast enough with the separation $\boldsymbol{x}-\boldsymbol{y}$, then $P_{\boldsymbol{k}}$'s are smooth or even analytic functions of $\boldsymbol{k}$ [1]. In this case, the Chern number [2]:

$$\mathrm{Ch}(P) = 2\pi\imath\epsilon^{\alpha\beta} \int_{\mathbb{T}^2} \frac{\mathrm{d}\boldsymbol{k}}{(2\pi)^2}\, \mathrm{tr}\big(P_{\boldsymbol{k}}\, \partial_{k_\alpha} P_{\boldsymbol{k}}\, \partial_{k_\beta} P_{\boldsymbol{k}}\big) \tag{2}$$

is well defined and takes only quantized values. Above, "tr" refers to the trace over the local orbital degrees of freedom. This expression can be written in real-space using Eq. (1):

$$\mathrm{Ch}(P) = -2\pi\imath\epsilon^{\alpha\beta}\mathcal{T}\big(P\,[P, X_\alpha][P, X_\beta]\big), \tag{3}$$

where $\mathcal{T}$ refers to the trace per volume $\lim_{V\to\infty} \frac{1}{V}\mathrm{Tr}_V\{\cdot\}$, equal to $\int_{\mathbb{T}^2} \frac{\mathrm{d}\boldsymbol{k}}{(2\pi)^2}$ for translational invariant systems, and $\boldsymbol{X}$ is the position operator. One remarkable fact is that (3) remains stable and quantized even in the presence of strong disorder when the spectral gap is closed, provided the matrix elements $\langle \boldsymbol{x}|P|\boldsymbol{y}\rangle$ continue to display a fast decay, more precisely if:

$$\sum_{\boldsymbol{y}\in\mathbb{Z}^2} |\boldsymbol{x}-\boldsymbol{y}|^2 \big|\langle \boldsymbol{x}|P|\boldsymbol{y}\rangle\big|^2 \le \infty. \tag{4}$$

This happens to be the case for the Fermi projector of a non-interacting model when the Fermi level is located in a mobility gap [3], that is, whenever the diagonal components of the conductivity tensor vanish.

In the present work we are dealing with both disordered non-interacting and disordered interacting systems. For the former, the topology is encoded in the Fermi projection which projects onto the states below the Fermi level. For the latter, the projector which encoded the topology can be obtained from the two-point imaginary time Green's function:

$$G(\boldsymbol{x}, \boldsymbol{y}; \tau) = \langle \Psi_0 | c^\dagger_{\boldsymbol{x}}(\tau) c_{\boldsymbol{y}}(0) | \Psi_0 \rangle, \tag{5}$$

at zero frequency, as detailed in [4]. Its matrix elements are obtained from a Monte-Carlo simulation and the inverse of the resulting matrix plays the role of the one-particle Hamiltonian in non-interacting models. The equivalent of the Fermi projection is then obtained by filling the positive eigenvalues of this Hamiltonian. We define the topological invariant as the Chern number of this projector.

To evaluate (3), we follow the practical solution devised in the series of works [5–7]. The most difficult part of the problem is to represent or approximate the commutators $[X_j, F_\omega]$ for a disordered operator $F_\omega$ on a finite volume with periodic boundary conditions. Here, $\omega$ represents the disorder configuration and encodes all the random fluctuations in the Hamiltonian coefficients. Recall that on the infinite volume:

$$\langle \boldsymbol{x}|[X_j, F_\omega]|\boldsymbol{y}\rangle = (x_j - y_j)\langle \boldsymbol{x}|F_\omega|\boldsymbol{y}\rangle, \quad j = 1, 2, \tag{6}$$

and clearly the factor $x_j - y_j$ is antagonistic to the periodic boundary conditions. But here is a set of key observations:

- Typically, the kernels $\langle \boldsymbol{x}|F_\omega|\boldsymbol{y}\rangle$ decay exponentially with $|\boldsymbol{x}-\boldsymbol{y}|$, on average.
- When restricting $\boldsymbol{x}$ to a finite lattice $-N \leq x_j \leq N$, $j=1,2$, and imposing periodic boundary conditions, we are practically placing the system on the torus $\mathcal{C}_N \times \mathcal{C}_N$, where $\mathcal{C}_N$ is the circle of perimeter $2N+1$.
- The factor $x_j - y_j$ is indeed antagonistic to this circle but we only need to represent the factor exactly for $\boldsymbol{x}$ close to $\boldsymbol{y}$, which leaves plenty of room to make it compatible with the circle (i.e. periodic).

Based on these guiding principles, the following procedure was proposed in Ref. [7]. Let $f:[-1,1]\to\mathbb{R}$ be a smooth and periodic function such that $f(r)=r$, for $|r|$ smaller than some $\alpha \lesssim 1$. It is used to define a function on the circle $\mathcal{C}_N$: $f_N(x)=Nf(x/N)$, which has the correct periodicity and is equal to $x$ for $|x|<\alpha N$. Let us consider its discrete Fourier representation:

$$f_N(x) = \frac{1}{2N+1}\sum_\lambda c_\lambda \lambda^x, \tag{7}$$

where the sum is over all $2N+1$ solutions of the equation $z^{2N+1}=1$. This will enable us to extend the domain of this function indefinitely (note that this is indeed needed because $x_j - x_j'$ takes values in the interval $[-2N, 2N]$) and to finally define the proper replacement of the antagonistic factor in Eq. (6):

$$x_j - y_j \to \sum_\lambda c_\lambda \lambda^{x_j - y_j}. \tag{8}$$

From the above approximation, a concrete form of the approximating commutators can be derived. Numerically, we found that the periodicity of the starting function $f$ is not that important in practice, and in most of our calculations we simply use $f(r)=r$ over the entire $[-1,1]$ interval. In this case, the Fourier coefficients are known explicitly and given below.

To summarize, the canonical and optimal finite-volume approximation scheme that emerges from the above arguments consists of substituting the commutator $[X_j, F_\omega]$ with:

$$\lfloor X_j, \widetilde{F}_\omega \rfloor = \sum_{\lambda\neq 1} c_\lambda \lambda^{X_j} \widetilde{F}_\omega \lambda^{-X_j}, \quad c_\lambda = \frac{\lambda^{N+1}}{1-\lambda}, \tag{9}$$

where $\widetilde{F}_\omega$ represents the finite-volume approximation of $F_\omega$. Based on the key factors listed above, Ref. [7] established the following rigorous result. Let $\Phi_j$ be smooth functions and let the accent $\sim$ indicate the restriction to a finite volume. Then:

$$\left|\mathcal{T}\{[X_{\alpha_1}, \Phi_1(H_\omega)][X_{\alpha_2}, \Phi_2(H_\omega)]\ldots\} - \widetilde{\mathcal{T}}\{\lfloor X_{\alpha_1}, \Phi_1(\widetilde{H}_\omega)\rfloor \lfloor X_{\alpha_2}, \Phi_2(\widetilde{H}_\omega))\rfloor\ldots\}\right| < C_\Phi e^{-\gamma N}.$$

Based on this result, any correlation function involving localized observables and their commutators with the position operators can be canonically approximated on a finite volume, and this approximation converges exponentially fast to the thermodynamic limit. The above formulas were used to evaluate the spin Chern numbers of the Kane-Mele model, the DKM model, the DKMH model, the GKM model, and the GKMH model, all with disorder, studied in this work.

## THE GKM AND DKM MODELS

Here we provide the Hamiltonian expressions for the GKM and DKM models [8, 9] (generalizations of the well-known Kane-Mele model [10, 11]), including their effective low-energy theories. The GKM can be expressed in momentum space as [12],

$$H_{GKM} = \sum_{\mathbf{k}\in B.Z.} \Psi_\mathbf{k}^\dagger \left[ \begin{pmatrix} 0 & -tf(\mathbf{k}) - t_3 f_3(\mathbf{k}) \\ -tf^*(\mathbf{k}) - t_3 f_3^*(\mathbf{k}) & 0 \end{pmatrix} \otimes \mathbb{1}_{2\times 2} + \begin{pmatrix} 2\lambda_{so} g(\mathbf{k}) & 0 \\ 0 & -2\lambda_{so} g(\mathbf{k}) \end{pmatrix} \otimes \sigma_z \right] \Psi_\mathbf{k}, \tag{10}$$

where the basis $\Psi_\mathbf{k}^T \equiv (\Psi_\mathbf{k}^{\uparrow T}\ \Psi_\mathbf{k}^{\downarrow T}) = (c_{\mathbf{k}\uparrow}(A)\ c_{\mathbf{k}\uparrow}(B)\ c_{\mathbf{k}\downarrow}(A)\ c_{\mathbf{k}\downarrow}(B))$ with $\mathbf{k}$ denoting the momentum, $\uparrow, \downarrow$ the $z$-axis projections of the spin, and $A, B$ the sub lattice degrees of freedom shown in Fig. 1(a). Here $\sigma_z$ is the Pauli matrix for the spin degrees of freedom. The expressions $g(\mathbf{k}) \equiv -\sin(\mathbf{k}\cdot\mathbf{e}_1)+\sin(\mathbf{k}\cdot\mathbf{e}_2)+\sin[\mathbf{k}\cdot(\mathbf{e}_1-\mathbf{e}_2)]$, $f(\mathbf{k}) = 1+e^{i\mathbf{k}\cdot\mathbf{e}_1}+e^{i\mathbf{k}\cdot\mathbf{e}_2}$ and $f_3(\mathbf{k}) = e^{i\mathbf{k}\cdot(\mathbf{e}_1+\mathbf{e}_2)} + 2\cos[\mathbf{k}\cdot(\mathbf{e}_1-\mathbf{e}_2)]$, where $\mathbf{e}_1 = (1/2, \sqrt{3}/2)$ and $\mathbf{e}_2 = (-1/2, \sqrt{3}/2)$.

The B.Z. is shown in Fig. 1(b). In the KM-type models that we consider, a few momenta dominate the low-energy descriptions [12]. As a function of $t_3$, gap closings occur at the TRIM points located at $\mathbf{M}_{1,2} \equiv (\pm\pi, \pi/\sqrt{3})$ and $\mathbf{M}_3 \equiv (0, 2\pi/\sqrt{3})$. At the TRIM, the diagonal elements of the Hamiltonian matrices vanish, $g(\mathbf{M}_a) = 0$, and the band gaps in GKM are controlled by the off-diagonal elements, which are related to real-valued first and third neighbor hopping. The low-energy form (to quadratic order in the momentum, needed for the self-consistent Born approximation in the case of disorder) of the Hamiltonian near the three different $\mathbf{M}_a$ can be obtained by expanding $f(\mathbf{k}), f_3(\mathbf{k})$, and $g(\mathbf{k})$ as

$$f(\mathbf{M_1} + \delta\mathbf{k}) = 1 - i\delta k_x + \frac{\sqrt{3}}{2}\delta k_x \delta k_y, \tag{11}$$

$$f_3(\mathbf{M_1} + \delta\mathbf{k}) = -3 - i\sqrt{3}\delta k_y + \frac{3}{2}\delta k_y^2 + \delta k_x^2, \tag{12}$$

$$g(\mathbf{M_1} + \delta\mathbf{k}) = \sqrt{3}\delta k_y - \delta k_x, \tag{13}$$

$$f(\mathbf{M_2} + \delta\mathbf{k}) = 1 + i\delta k_x - \frac{\sqrt{3}}{2}\delta k_x \delta k_y, \tag{14}$$

$$f_3(\mathbf{M_2} + \delta\mathbf{k}) = -3 - i\sqrt{3}\delta k_y + \frac{3}{2}\delta k_y^2 + \delta k_x^2, \tag{15}$$

$$g(\mathbf{M_2} + \delta\mathbf{k}) = -\sqrt{3}\delta k_y - \delta k_x \tag{16}$$

$$f(\mathbf{M_3} + \delta\mathbf{k}) = -1 - i\sqrt{3}\delta k_y + \frac{3}{4}\delta k_y^2 + \frac{1}{4}\delta k_x^2, \tag{17}$$

$$f_3(\mathbf{M_3} + \delta\mathbf{k}) = 3 + i\sqrt{3}\delta k_y - \frac{3}{2}\delta k_y^2 - \delta k_x^2, \tag{18}$$

$$g(\mathbf{M_3} + \delta\mathbf{k}) = 2\delta k_x. \tag{19}$$

The low-energy forms of the GKM model for the various $\mathbf{M}_a$ points are given by

$$H^{eff}_{GKM}(\mathbf{M_1} + \delta\mathbf{k}) = \begin{pmatrix} 2\sqrt{3}\lambda\delta k_y - 2\lambda\delta k_x & -t + 3t_3 + i(\sqrt{3}t_3\delta k_y + t\delta k_x) + p_1(\delta\mathbf{k}) \\ -t + 3t_3 - i(\sqrt{3}t_3\delta k_y + t\delta k_x) + p_1(\delta\mathbf{k}) & -2\sqrt{3}\lambda\delta k_y + 2\lambda\delta k_x \end{pmatrix}, \tag{20}$$

$$H^{eff}_{GKM}(\mathbf{M_2} + \delta\mathbf{k}) = \begin{pmatrix} -2\sqrt{3}\lambda\delta k_y - 2\lambda\delta k_x & -t + 3t_3 + i(\sqrt{3}t_3\delta k_y - t\delta k_x) + p_2(\delta\mathbf{k}) \\ -t + 3t_3 - i(\sqrt{3}t_3\delta k_y - t\delta k_x) + p_2(\delta\mathbf{k}) & 2\sqrt{3}\lambda\delta k_y + 2\lambda\delta k_x \end{pmatrix}, \tag{21}$$

$$H^{eff}_{GKM}(\mathbf{M_3} + \delta\mathbf{k}) = \begin{pmatrix} 4\lambda\delta k_x & t - 3t_3 + i\sqrt{3}(t - t_3)\delta k_y + p_3(\delta\mathbf{k}) \\ t - 3t_3 - i\sqrt{3}(t - t_3)\delta k_y + p_3(\delta\mathbf{k}) & -4\lambda\delta k_x \end{pmatrix}, \tag{22}$$

where $p_1(\delta\mathbf{k}) = -\frac{3}{2}t_3\delta k_y^2 - \frac{\sqrt{3}}{2}t\delta k_y\delta k_x - t_3\delta k_x^2$, $p_2(\delta\mathbf{k}) = -\frac{3}{2}t_3\delta k_y^2 + \frac{\sqrt{3}}{2}t\delta k_y\delta k_x - t_3\delta k_x^2$, and $p_3(\delta\mathbf{k}) = -\frac{3}{4}(t - 2t_3)\delta ky^2 - \frac{1}{4}(t - 4t_3)\delta k_x^2$ are the quadratic contributions to the off-diagonal matrix elements that will play an important role in the self-consistent Born approximation used to study the disordered case. It is evident that the gap at all three $\mathbf{M}_a$ is given by $|t - 3t_3|$, though the sign is different for the $\mathbf{M_3}$ point relative to the $\mathbf{M_1}$ and $\mathbf{M_2}$ points [12]. Note also that the gap is controlled by the terms proportional to $\tau^x$ in the basis of the two bands, rather than $\tau^z$, as occurs in the Kane-Mele model where the gap closings are located at the $K$ and $K'$ points. This fact has important implications for how different types of disorder (bond and on-site) will renormalize the effective masses (gaps) at the low-energy points of the theory [13].

The DKM model can be expressed in momentum space as [12],

$$H_{DKM} = \sum_{\mathbf{k}\in B.Z.} \Psi^\dagger_{\mathbf{k}} \left[ \begin{pmatrix} 0 & -t_d - tf_d(\mathbf{k}) \\ -t_d - tf_d^*(\mathbf{k}) & 0 \end{pmatrix} \otimes \mathbb{1}_{2\times 2} + \begin{pmatrix} 2\lambda_{so}g(\mathbf{k}) & 0 \\ 0 & -2\lambda_{so}g(\mathbf{k}) \end{pmatrix} \otimes \sigma_z \right] \Psi_{\mathbf{k}}, \tag{23}$$

where $f_d(\mathbf{k}) = e^{i\mathbf{k}\cdot\mathbf{e}_1} + e^{i\mathbf{k}\cdot\mathbf{e}_2}$. When we vary the dimerized hopping amplitude $t_d$ while fixing $t$, the band gap only closes at $\mathbf{M}_3$ due to the breakdown of $C_3$ rotational symmetry. Similar to the GKM, the band gap at the TRIM ($\mathbf{M}_3$) is controlled by the off-diagonal terms since $g(\mathbf{M}_3) = 0$. The low-energy form of the DKM Hamiltonian near $\mathbf{M}_3$ can be obtained from

$$f_d(\mathbf{M_3} + \delta\mathbf{k}) = -2 - i\sqrt{3}\delta k_y + \frac{3}{4}\delta k_y^2 + \frac{1}{4}\delta k_x^2, \tag{24}$$

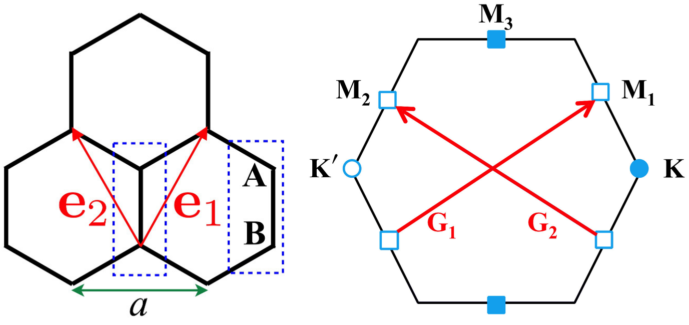


FIG. 1. (a) Schematic of the honeycomb lattice with two sublattices labeled $A$ and $B$. The vectors $\mathbf{e}_{1/2} = (\pm 1/2, \sqrt{3}/2)$ connect the same sublattice in different unit cells. The lattice constant $a$ is set to 1. (b) Illustration of the Brillouin zone (B.Z.). There are several relevant momenta that are important in the low-energy descriptions of variants of KM models–The usual momenta $\mathbf{K} = -\mathbf{K}' = (4\pi/3, 0)$ as the locations of the Dirac nodes in the original KM model and the time-reversal-invariant momenta (TRIM) $\mathbf{M}_{1,2} \equiv (\pm\pi, \pi/\sqrt{3})$ and $\mathbf{M}_3 \equiv (0, 2\pi/\sqrt{3})$. Note that $\mathbf{M}_1$ and $\mathbf{M}_2$ are related by $C_3$ lattice rotation symmetry. $\mathbf{G}_1$ and $\mathbf{G}_2$ are the reciprocal lattice vectors.

which yields

$$H^{eff}_{DKM}(\mathbf{M_3} + \delta\mathbf{k}) = \begin{pmatrix} 4\lambda\delta k_x & 2t - t_d + i\sqrt{3}t\delta k_y - \frac{1}{4}t(3\delta k_y^2 + \delta k_x^2) \\ 2t - t_d - i\sqrt{3}t\delta k_y - \frac{1}{4}t(3\delta k_y^2 + \delta k_x^2) & -4\lambda\delta k_x \end{pmatrix}, \tag{25}$$

so that the gap at the $\mathbf{M}_3$ point is given by $|-t_d + 2t|$. In the main text of this paper, we use the relation $t_d = t + \delta t_d$, so the modification of the KM model to the DKM model has an additional $\delta t_d$ along the $\hat{e}_3 = (\hat{e}_1 + \hat{e}_2)/|\hat{e}_1 + \hat{e}_2|$ direction.

## THE SELF-CONSISTENT BORN APPROXIMATION (SCBA)

We follow the notation of Refs.[13, 14]. In contrast to earlier studies [13–16] of disordered models with topological phases that had gap closings at either the $\Gamma$ point or the $K, K'$ points, the GKM model has gap closings at the three $\mathbf{M_a}$ points [8, 9], and the DKM model at the $\mathbf{M_3}$ point [9, 12]. As described in the section above, when the Hamiltonian is written in the basis (for a fixed spin orientation) of $H_0(\mathbf{k}) = h_0(\mathbf{k})\tau_0 + h_x(\mathbf{k})\tau_x + h_y(\mathbf{k})\tau_y + h_z(\mathbf{k})\tau_z$, it is the $\tau_x$ component that controls the gap. In the SCBA the (momentum-independent) self-energy, $\Sigma$, is computed from

$$\Sigma(E^+) = \frac{W^2}{12}\left(\frac{a}{2\pi}\right)^2 \int_{\mathrm{BZ}} d^2k \left[\tau_d(E^+\mathbb{1} - H_0 - \Sigma(E^+))^{-1}\tau_d\right], \tag{26}$$

where $E^+ = E_F + i\eta$ with $\eta > 0$ an infinitesimal, $W$ is the width of the random portion of the one body terms drawn from $[-W/2, W/2]$, and $\tau_d = \tau_x$ if the disorder is on the hopping terms and $\tau_d = \tau_0$ if the disorder is on-site [13], as in the conventional study of Anderson localization.

As pointed out in Ref.[13], if the mass gap is controlled by $\tau_z$ as it is at the $\Gamma$ point or the $K, K'$ points, then hopping and on-site disorder terms have an opposite effect on the self-energy since $\tau_x\tau_z\tau_x = -\tau_z$, while $\tau_0\tau_z\tau_o = +\tau_z$. However, if the mass gap is controlled by the $\tau_x$ piece of $H_0$ as it is for the GKM and DKM models: $H_0(\mathbf{M_a}) = M\tau_x$, then hopping and on-site disorder have the same effect since $\tau_x\tau_x\tau_x = +\tau_x$ and $\tau_0\tau_x\tau_0 = +\tau_x$, a new feature of the GKM and DKM models compared to earlier studies. The mass at the $\mathbf{M_a}$ points are then renormalized as,

$$\bar{M} = M + \Sigma_x(E = 0^+), \tag{27}$$

and the chemical potential is renormalized as

$$\mu = E_F - \Sigma_0(E = 0^+). \tag{28}$$

Approximate forms [13, 14] for the renormalized mass gap and chemical potential can be found by neglecting the self-energy in the integrand on the right-hand side of Eq.(26),

$$\Sigma(E^+) \approx \frac{W^2}{12}\left(\frac{a}{2\pi}\right)^2 \int_{\mathrm{BZ}} d^2k \left[\tau_d(E^+\mathbb{1} - H_0)^{-1}\tau_d\right]. \tag{29}$$

For a given spin projection, the Hamiltonian matrix $H_0$ is $2\times 2$, so that we may write (for $h_0(\mathbf{k})\equiv 0$, as is appropriate for our models),

$$(E^+\mathbb{1}-H_0)^{-1}=\frac{1}{(E^+)^2-\vec{h}(\mathbf{k})\cdot\vec{h}(\mathbf{k})}\left(E^+\mathbb{1}+H_0\right), \tag{30}$$

where $\vec{h}(\mathbf{k})=(h_x(\mathbf{k}),h_y(\mathbf{k}),h_z(\mathbf{k}))$. Thus, an approximate form for the mass and chemical potential contributions to the self-energy are,

$$\Sigma_x(E^+)\approx +\frac{W^2}{12}\left(\frac{a}{2\pi}\right)^2\int_{\mathrm{BZ}}d^2k\frac{h_x(\mathbf{k})}{(E^+)^2-\vec{h}(\mathbf{k})\cdot\vec{h}(\mathbf{k})}, \tag{31}$$

and

$$\Sigma_0(E^+)\approx +\frac{W^2}{12}\left(\frac{a}{2\pi}\right)^2\int_{\mathrm{BZ}}d^2k\frac{E^+}{(E^+)^2-\vec{h}(\mathbf{k})\cdot\vec{h}(\mathbf{k})}, \tag{32}$$

where the expressions Eq.(31) and Eq.(32) are independent of whether $\tau_d=\tau_0$ for on-site disorder, or $\tau_d=\tau_x$ for hopping disorder. From the low-energy expression of the GKM model, Eq.(20), Eq.(21), Eq.(22), and the DKM model, Eq.(25), we have $E^+=0$ for a half-filled particle-hole symmetric state. Hence, $\Sigma_0(E^+=0)\equiv 0$ and the chemical potential is *not* renormalized, according to Eq.(28).

We thus focus on the mass renormalization due to the disorder potential in the particle-hole symmetric state,

$$\Sigma_x(E^+=0^+)\approx -\frac{W^2}{12}\left(\frac{a}{2\pi}\right)^2\int_{\mathrm{BZ}}d^2k\frac{h_x(\mathbf{k})}{\vec{h}(\mathbf{k})\cdot\vec{h}(\mathbf{k})-(0^+)^2}, \tag{33}$$

which has its dominant contributions around $\mathbf{k}$ values where the denominator is smallest–namely around the $\mathbf{M_a}$ points. For both the GKM and the DKM models, the Hamiltonian is proportional to $\tau_x$ alone (at the $\mathbf{M_a}$ points), so if we neglect the momentum dependence of $h(\mathbf{k})$ and set it equal to the mass $M$, then we have $\Sigma(E^+=0^+)_x\approx -\frac{W^2}{12}\left(\frac{a}{2\pi}\right)^2\int_{\approx\mathbf{M_a}}d^2k\frac{1}{M}$ which will have the opposite sign as $M$ itself. However, one is not guaranteed that the integral is dominated by $\mathbf{k}\approx 0$. It turns out that the momentum dependence of $\vec{h}(\mathbf{k})$ is critical to obtain a the correct sign of the mass renormalization. In particular, it is the quadratic dependence contained in the functions $p_1(\mathbf{k}),p_2(\mathbf{k}),p_3(\mathbf{k})$ [see Eqs.(20)-(22)] and the quadratic terms proportional to $\tau_x$ in Eq.(25) that are responsible for the sign changes of the masses around any particular $\mathbf{M_a}$ point.

Provided there is a mass gap around each of the $\mathbf{M_a}$ points, one can neglect the $(0^+)^2$ in Eq.(33) so that the denominator of the integrand is manifestly positive. The correct sign of $\Sigma_x(E^+=0^+)$ relative to $M$ will come from $h_x(\mathbf{k})$, and the structure of the low-energy form of the GKM and DKM Hamiltonians implies it is the quadratic terms that are critical for obtaining the correct sign change. Unfortunately, because the dispersions around the $\mathbf{M_a}$ points are not isotropic, it is not possible to obtain simple closed analytical forms (for general parameters) for the leading corrections to $\Sigma_x$ as could be done for the Bernevig-Hughes-Zhang model [14] or the Kane-Mele model [13]. However, in special cases, closed analytical forms are available.

Around the $\mathbf{M_3}$ point the DKM model can be written as $H^{eff}_{DKM}(\mathbf{k})=[(2t-t_d)-\frac{1}{4}t(k_x^2+3k_y^2)]\tau_x-\sqrt{3}tk_y\tau_y+4\lambda k_x\tau_z$, so that the integral in Eq.(33) may be written as

$$\Sigma_x(E^+=0^+)\approx -\frac{W^2}{12}\left(\frac{a}{2\pi}\right)^2\int_{\approx\mathbf{M_3}}dk_xdk_y\frac{(2t-t_d)-\frac{1}{4}t(k_x^2+3k_y^2)}{[(2t-t_d)-\frac{1}{4}t(k_x^2+3k_y)^2]^2+16\lambda^2k_x^2+3t^2k_y^2}, \tag{34}$$

which can be simplified by rescaling $\tilde{k}_y=\sqrt{3}k_y$ and choosing $\lambda=t/2$ (in our numerical calculations, we assumed $\lambda=.4t$) so that the integral becomes spherically symmetric,

$$\Sigma_x(E^+=0^+)\approx -\frac{W^2}{12}\left(\frac{a}{2\pi}\right)^2\frac{1}{\sqrt{3}}\int_{\approx\mathbf{M_3}}d^2k\frac{\alpha+\beta k^2}{\alpha^2+\delta k^2+\beta^2k^4} \tag{35}$$

$$\approx -\frac{W^2}{12}\left(\frac{a}{2\pi}\right)^2\frac{2\pi}{2\sqrt{3}}\int_0^{\pi\hbar/a}du\frac{\alpha+\beta u}{\alpha^2+\delta u+\beta^2u^2}, \tag{36}$$

where $\alpha=(2t-t_d),\beta=-t/4$, and $\delta=tt_d/2$. This then gives a leading logarithmic contribution of

$$\Sigma_x(E^+=0^+)\approx -\frac{W^2a^2}{24\sqrt{3}\pi}\frac{1}{\beta}\log\left|\frac{\beta^2}{\alpha^2}\left(\frac{\pi\hbar}{a}\right)^4\right|. \tag{37}$$

The mass gap is $M = \alpha = (2t - t_d)$, which then always has a *positive* contribution since $\beta < 0$. Since the topological phase of the DKM model has $\alpha = (2t - t_d) > 0$, the disorder always tends to *stabilize* the topological phase, and may even drive a trivial state with $2t < t_d$ into a topological state, as our numerical calculations show. Our numerical calculations are based on a fully self-consistent numerical solution of Eq.(26).

For the GKM model the self-energy cannot generally be cast into the form of Eq.(36) (even for special parameter values), though the physics is essentially the same as an in the DKM model. Critically, the effect of the disorder is to drive all three mass terms (at the three $\mathbf{M_a}$ points) to change their sign in the direction of the topological phase, regardless of whether the parameters in the clean limit put the Hamiltonian in the topological or trivial phase. Our numerical calculations for the GKM are also based on a fully self-consistent numerical solution of Eq.(26).

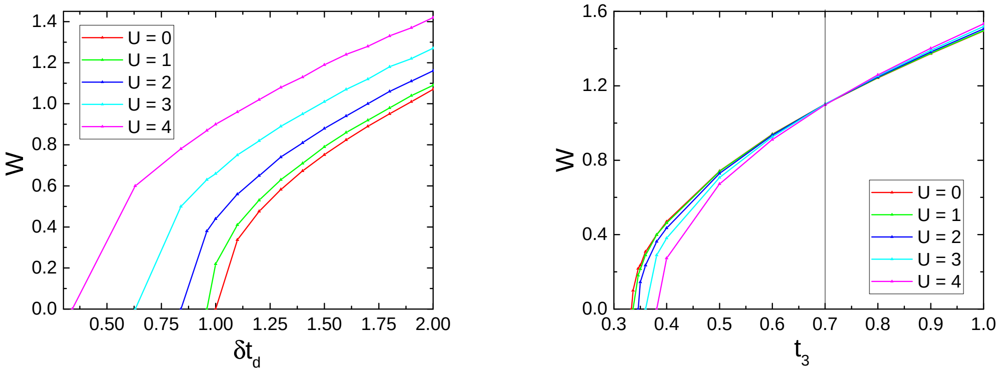


FIG. 2. Influence of disorder and interactions on the phase diagram of the DKM and GKM models. Left: The DKM model. Interactions tend to push the phase boundary into the topological regime while enlarging the trivial regime, while disorder tends to push the phase boundary into the trivial regime while enlarging the topological regime. Right: The GKM model. In contrast to the DKM model, both the interactions and the disorder tend to stabilize (enlarge) the topological region of the phase diagram, which is the region "above" the curves (for any given value of $U$).

## SIMULTANEOUS TREATMENT OF INTERACTIONS AND DISORDER (PERTURBATIVE)

In our work, we perform Monte Carlo simulations of interacting, disordered, fermion-sign problem free models (DKMH and GKMH models) with $Z_2$ topological insulator phases in their phase diagrams. We were interested in exploring the interplay of topology, interactions, and disorder on an equal footing. The QMC calculations are most stable for moderate interaction strengths, $U$, but we are able to analytically study the weak interaction limits using perturbation theory (in the interactions) combined with mean-field theory to obtain a renormalized band structure [12, 17].

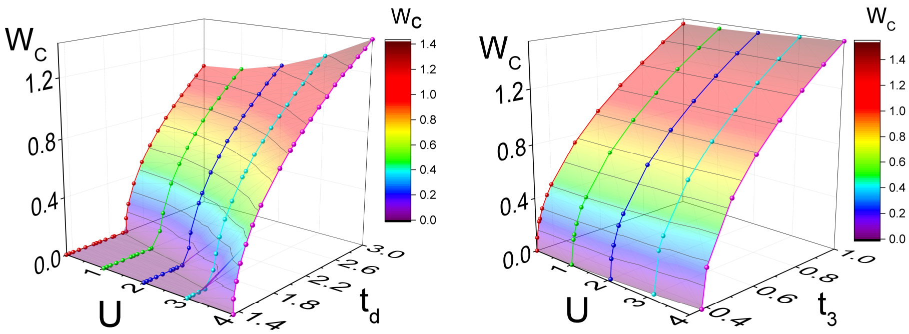


FIG. 3. Influence of disorder and interactions on the phase diagram of the DKM and GKM models computed using the self-consistent Born approximation (SCBA), Eq.(41) and Eq.(38). The region "above" the surface is a $Z_2$ topological insulator, and the region "below" it is a trivial insulator.

In Refs.[12, 17], it was shown that the parameters of the GKMH model are renormalized as

$$t \rightarrow t + U^2(\chi_1)^3, \quad (38)$$
$$t_3 \rightarrow t_3 + U^2(\chi_3)^3, \quad (39)$$
$$(40)$$

where $\chi_1$ is the expectation value of the nearest neighbor hopping in the presence of interactions, and $\chi_3$ is the expectation value of the third neighbor hopping in the presence of interactions. This leads to a renormalized gap of $\Delta_G = t - 3t_3 + U^2((\chi_1)^3 - 3(\chi_3)^3)$. For $t \approx 3t_3$, one has $\chi_1 = 0.20705$ and $\chi_3 = 0.03064$, so that the correction to the gap is $0.00879U^2$. The positive sign of this term tends to stabilize the topological state [12, 17].

In Refs.[12, 17], it was shown that the parameters of the DKMH model are renormalized as

$$t \rightarrow t + U^2(\chi_1)^3, \quad (41)$$
$$t_d \rightarrow t_d + U^2(\chi_1^d)^3, \quad (42)$$
$$(43)$$

where $\chi_1$ is the expectation value of the nearest neighbor hopping in the presence of interactions, and $\chi_1^d$ is the expectation value of the modified first neighbor hopping in the presence of interactions. This leads to a renormalized gap of $\Delta_D = 2t - t_d - U^2((\chi_1^d)^3 - 2(\chi_1)^3)$. For $t \approx 2t_d$, one has $\chi_1 = 0.15770$ and $\chi_1^d = 0.36627$, so that the correction to the gap is $-0.04129U^2$. The negative sign of this term tends to destabilize the topological state [12, 17].

## QUANTUM MONTE CARLO CALCULATIONS OF GKMH AND DKMH MODELS

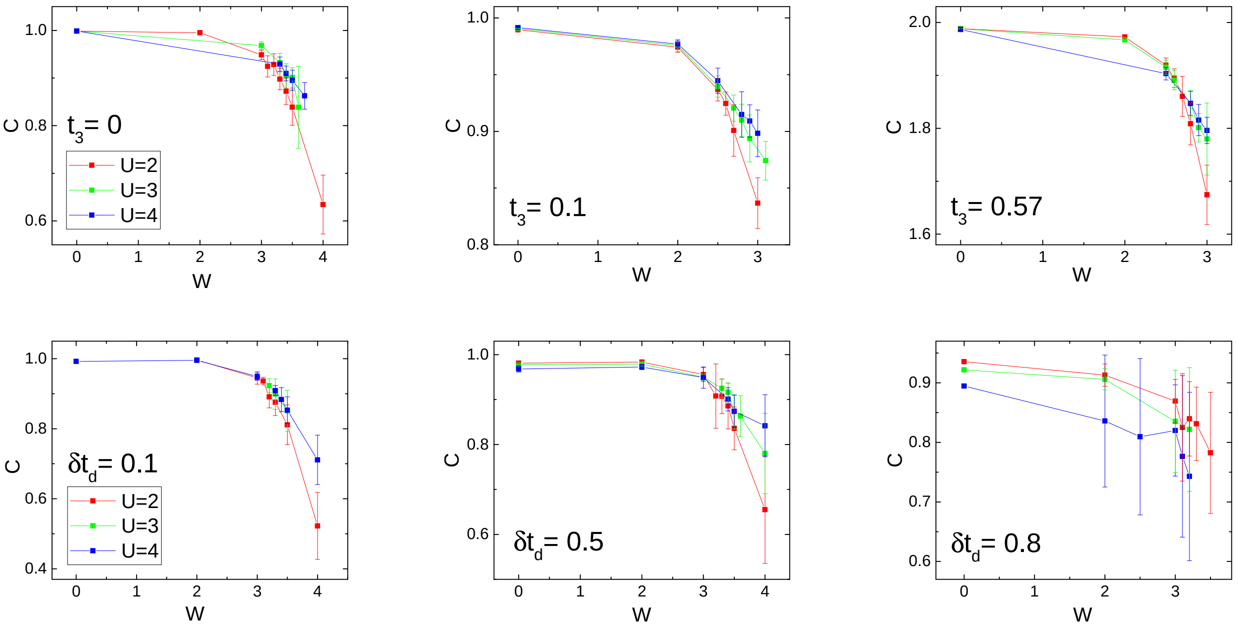


FIG. 4. QMC calculations for spin Chern numbers at different interaction strengths, $U = 2, 3, 4$. Between 10 and 30 disorder realizations are averaged over. The top panels show the disorder dependence of the spin Chern number for different values of the one-body tuning parameter $t_3$ for the GKMH model, and the bottom panels show the disorder dependence of the spin Chern number for different values of the one-body tuning parameter $\delta t_d$ for the DKMH model.

We use the quantum Monte Carlo techniques as described in Ref.[4, 8, 9, 12] to compute the single-particle Greens in real space for each disorder realization. From the zero frequency real-space Greens' function, we use the results from the first section of the supplemental material to obtain a highly accurate value for the spin-Chern number. In our calculations, for each interaction value $U$, we used between 10 and 30 disorder realizations on a $12 \times 12$ lattice.

Smaller $6 \times 6$ sizes could not give accurate results, and $18 \times 18$ was beyond our computational capability. Our main results are shown in Fig.4.

We use the results of Fig.4 to determine the critical disorder strength, $W_c$, for each model using a "peel off" criterion: When the Chern number decreases by 10% with respect to the $W = 0$ limit, this value is identified as the critical disorder strength for that particular value of $U$ and $t_3$ or $\delta t_d$. These critical values for the two models are summarized in the top panel of Fig.2 of the main text. For the GKMH model there is a quantum phase transition near $t_3 = 1/3$ (the critical $t_3^c$ depends on the $U$ value, as shown in the lower panel of Fig.2 of the main text), where the spin Chern number in the clean limit changes from 1 for $0 < t_3 < t_3^c$ to 2 for $t_3 > t_3^c$. This is evident in the figures in the upper panel of Fig.4. For the DKMH there is quantum phase transition near $\delta t_d = 1$ (the critical $\delta t_d^c$ depends on the $U$ value, as shown in the lower panel of Fig.2 of the main text), where the spin Chern number in the clean limit changes from 1 for $0 < \delta t_d < \delta t_d^c$ to 0 for $\delta t_d > \delta t_d^c$. Since there is no transition with disorder in the spin Chern number for $\delta t_d > \delta t_d^c$ we do not consider this case. Note that near the transition, where $\delta t_d = 0.8$, the fluctuations in the spin Chern number are large. This prevents us from an accurate determination of the critical value of W near phase boundaries. In addition, our inability to compute larger size lattices also prevents a finite scaling analysis that would help provide a more accurate $W_c$ in the thermodynamic limit.


[1] M. Reed and B. Simon, *Methods of Modern Mathematical Physics. Vol II. Fourier Analysis, Self-adjointness* (Academic Press, New York, 1975).
[2] J. E. Avron, L. Sadun, J. Segert, and B. Simon, Comm. Math. Phys. **124**, 595 (1989).
[3] J. Bellissard, A. van Elst, and H. Schulz-Baldes, J. Math. Phys. **35**, 5373 (1994).
[4] Zi Yang Meng, Hsiang-Hsuan Hung, Thomas C. Lang, *The characterization of topological properties in Quantum Monte Carlo simulations of the Kane-Mele-Hubbard model*, Mod. Phys. Lett B **28**, 143001 (2014).
[5] T. H. E. Prodan and B. Bernevig, Phys. Rev. Lett. **105**, 115501 (2010).
[6] E. Prodan, J. Phys. A: Math. Theor. **44**, 113001 (2011).
[7] E. Prodan, Appl. Math. Res. Express AMRX **2013**, 176 (2013).
[8] H.-H. Hung, L. Wang, Z.-C. Gu, and G. A. Fiete, Phys. Rev. B **87**, 121113 (2013).
[9] H.-H. Hung, V. Chua, L. Wang, and G. A. Fiete, Phys. Rev. B **89**, 235104 (2014).
[10] C. L. Kane and E. J. Mele, Phys. Rev. Lett. **95**, 146802 (2005).
[11] C. L. Kane and E. J. Mele, Phys. Rev. Lett. **95**, 226801 (2005).
[12] H.-H. Lai and H.-H. Hung, International Journal of Modern Physics B **29**, 1530005 (2015).
[13] J. Song, H. Liu, H. Jiang, Q.-F. Sun, and X. C. Xie, Phys. Rev. B **85**, 195125 (2012).
[14] C. W. Groth, M. Wimmer, A. R. Akhmerov, J. Tworzydło, and C. W. J. Beenakker, Phys. Rev. Lett. **103**, 196805 (2009).
[15] H. Jiang, L. Wang, Q.-F. Sun, and X. C. Xie, Phys. Rev. B **80**, 165316 (2009).
[16] J. Li, R.-L. Chu, J. K. Jain, and S.-Q. Shen, Phys. Rev. Lett. **102**, 136806 (2009).
[17] H.-H. Lai, H.-H. Hung, and G. A. Fiete, Phys. Rev. B **90**, 195120 (2014).
